# Supplementary material for: A Unified Interactive Model Evaluation for Classification, Object Detection, and Instance Segmentation in Computer Vision
Source: arXiv:2308.05168 source file (2023-08-09)
Supplement: Supplementary file 1 [file Appendix.pdf]

# Appendix A: Survey on Computer Vision Model Evaluation

## Part One: Basic Information

1. Please select the range of your age. [Select one of the following]

- ☐ 11-20
- ☐ 21-30
- ☐ 31-40
- ☐ 41-50
- ☐ 51-60
- ☐ 60+

2. Please select your gender. [Select one of the following]

- ☐ Male
- ☐ Female

3. How many years of experience do you have in computer vision? [Select one of the following]

- ☐ less than 1 year
- ☐ 1-3 years
- ☐ 3-5 year
- ☐ 41-50
- ☐ 51-60
- ☐ 60+

## Part Two: Current Practice

4. What computer vision tasks do you work with? [Select all that apply]

- ☐ Image classification
- ☐ Object detection
- ☐ Image segmentation
- ☐ Other: \_\_\_\_\_

5. What stage of machine learning do you typically work on? [Select all that apply]

- ☐ Data collection and processing
- ☐ Data labeling
- ☐ Model training
- ☐ Model evaluation

6. Have you ever worked with multiple tasks (e.g., classification, detection, segmentation) in one application? If so, how many tasks did you work with? [Select one of the following]

- ☐ No
- ☐ 2
- ☐ 3

- ☐ 4
- ☐ 4+

**7. How do you evaluate a computer vision model? [Select all that apply]**

- ☐ By analyzing the training logs of the model, including \_\_\_\_\_
- ☐ By using visualization tools, including \_\_\_\_\_
- ☐ By inspecting the prediction results of a given sample
- ☐ Other: \_\_\_\_\_

**8. What problems do you encounter when using these evaluation methods? [Select all that apply]**

- ☐ These methods focus on evaluating classification results and do not support the evaluation of more complex prediction results, such as detection results
- ☐ Cannot help users identify problems in the training data, e.g., incorrect annotations
- ☐ Cannot help users identify the classes where the model performs poorly
- ☐ Cannot help users compare different models at the class level and instance level
- ☐ Other: \_\_\_\_\_

**Part Three: Key Features Needed**

Do you think the following features can help you analyze and improve computer vision model performance? Please rate the importance.

Unimportant / Slightly important / Moderately important / Important / Very important

**9. A unified evaluation for different computer vision tasks.**

Unimportant ☐ — ☐ — ☐ — ☐ — ☐ Very important

**10. Analyzing the overall model performance on the entire dataset.**

Unimportant ☐ — ☐ — ☐ — ☐ — ☐ Very important

**11. Analyzing the model performance on data subsets (e.g., objects with large/small sizes).**

Unimportant ☐ — ☐ — ☐ — ☐ — ☐ Very important

**12. Exploring the prediction results of a given sample (e.g., a mispredicted sample) efficiently.**

Unimportant ☐ — ☐ — ☐ — ☐ — ☐ Very important
